# Supplementary material for: On the Correlation between L Dwarf Optical and Infrared Variability and Radio Aurorae
Source: arXiv:2009.05590 source file (2020-09-11)
Supplement: Supplementary file 1 [file sec_appendix.tex]

\appendix\label{sec:appendix}

\section{KS test on the probability distributions of the occurrence rates.}

The Kolmogorov-Smirnov (KS) test is a frequentest, nonparametric test that can be used to assess how likely it is that two samples originate from the same distribution. It compares two empirical cumulative distribution functions by measuring the maximum distance between the two curves. The KS test is one of the more powerful tests for comparing two distributions since it does not assume any underlying shape of the distribution and takes into account both the locations and shapes of the empirical cumulative distribution functions. The KS test however cannot determine whether two samples are from the same distributions, but can only reject the null-hypothesis that two distributions are the same.

% \begin{wrapfigure}{R}{0.40\textwidth}
%     \centering
%     \includegraphics[width=\linewidth]{images/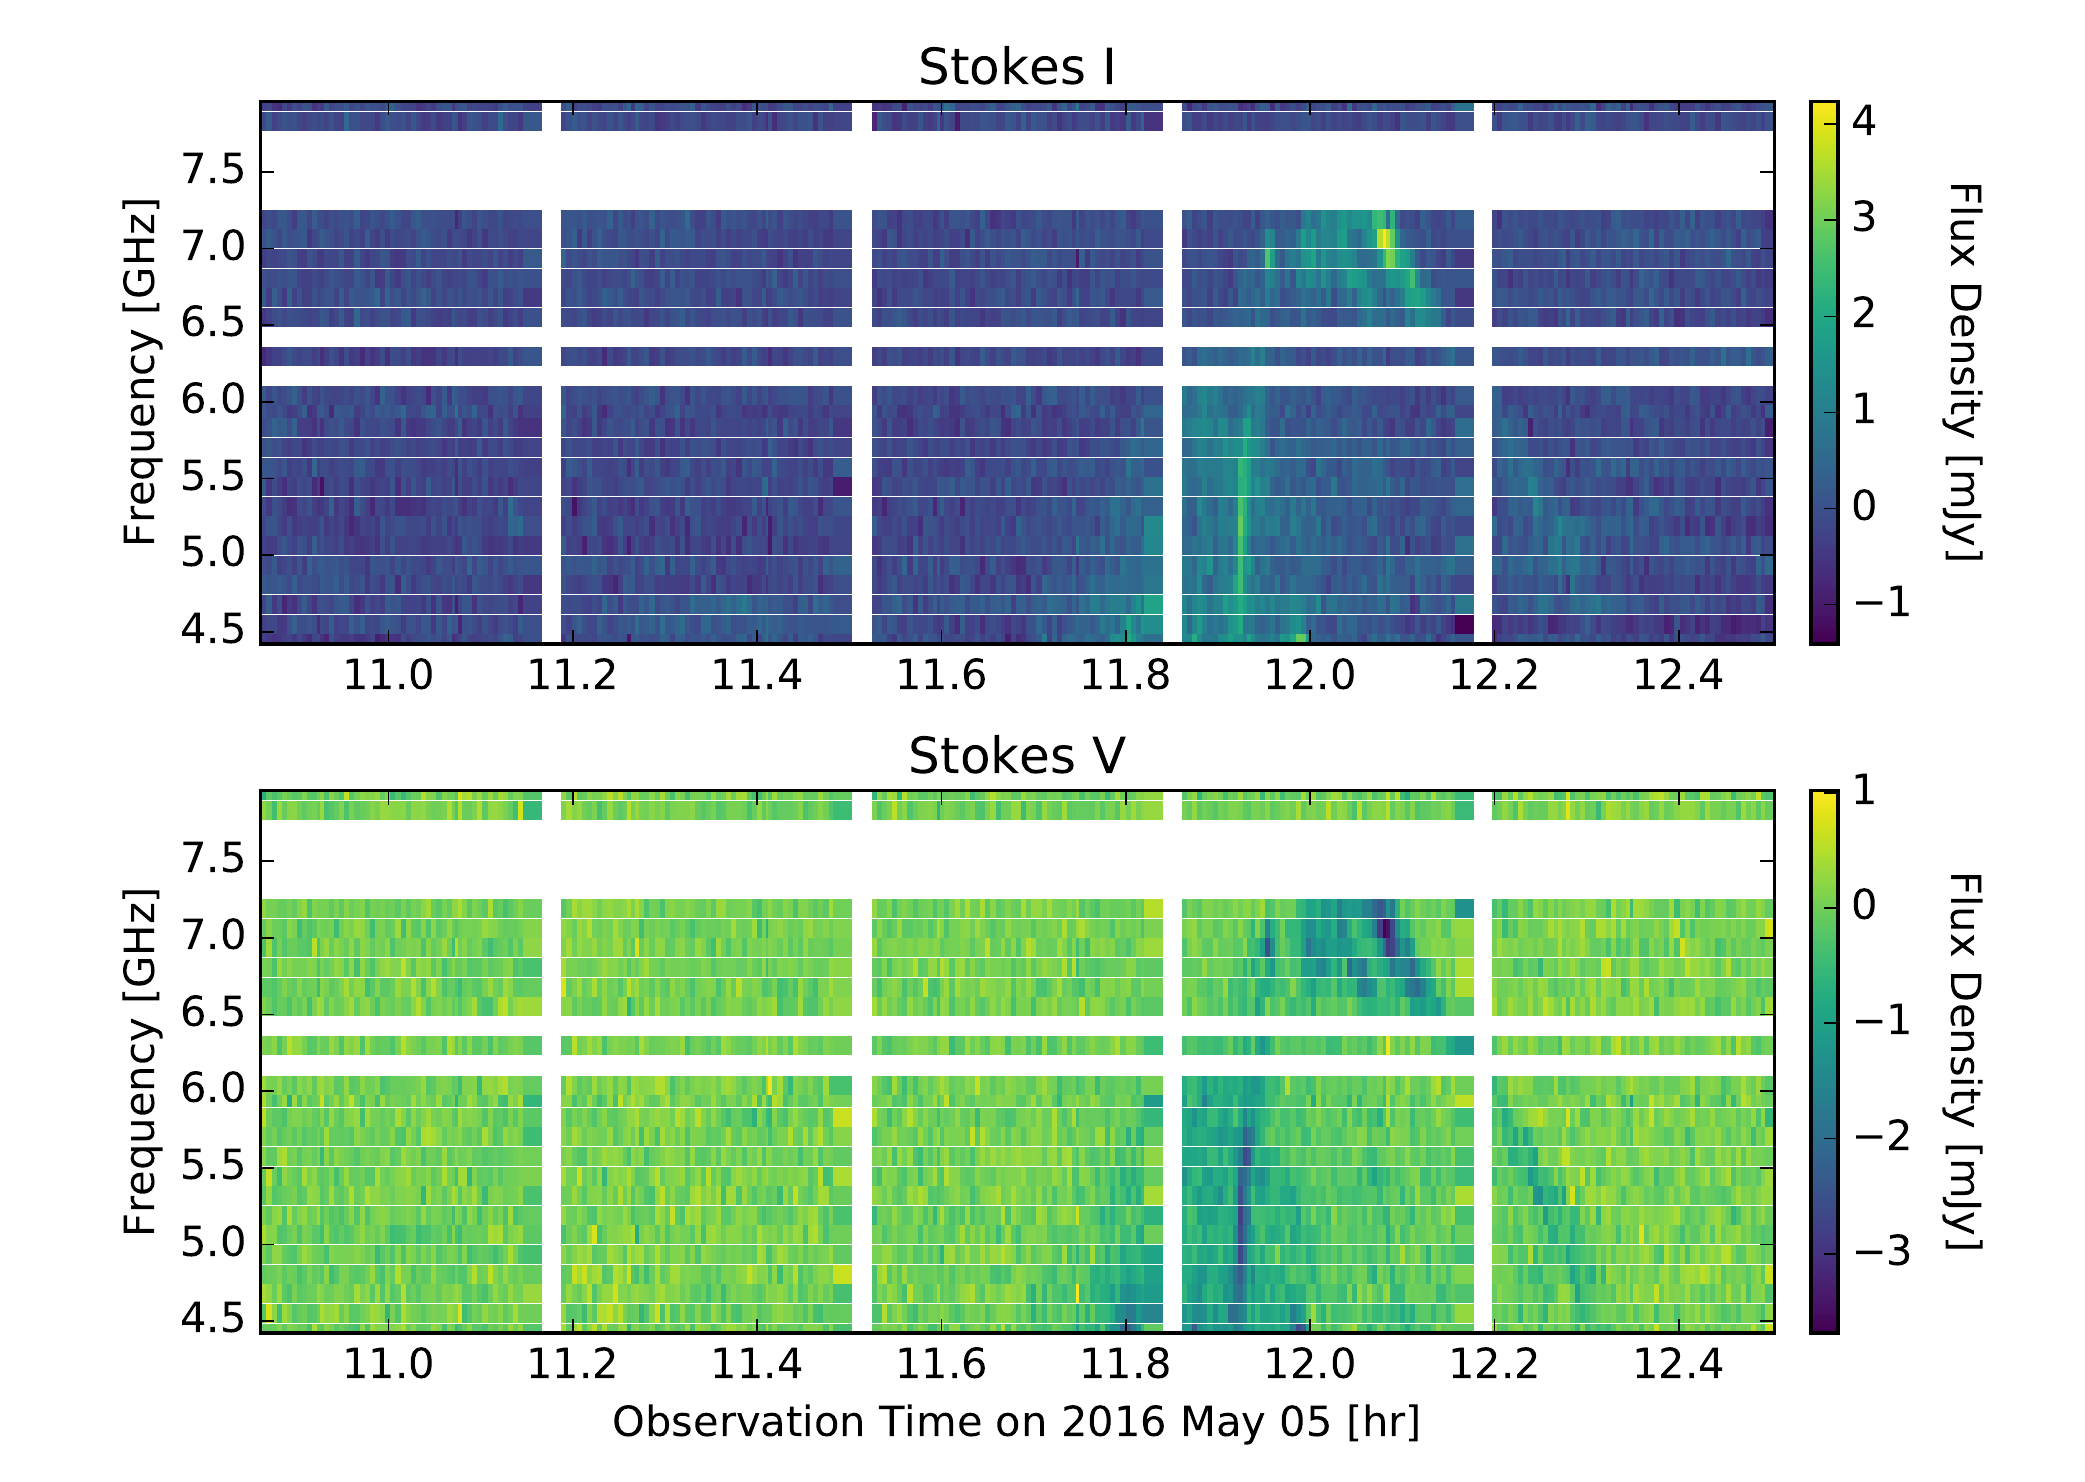}
%     \caption{The occurrence rate distributions from the results of our calculation (solid lines) overlaid on histograms of the empirically drawn occurrence rates to set up the KS test. The bin sizes are arbitrary and for plotting purposes only.}
%     \label{fig:ks}
% \end{wrapfigure}

\begin{figure}[t]
    \centering
    \includegraphics[width=0.5\linewidth]{images/figure_2.pdf}
    \caption{The occurrence rate distributions from the results of our calculation (solid lines) overlaid on histograms of the empirically drawn occurrence rates to set up the KS test. The bin sizes are arbitrary and for plotting purposes only.}
    \label{fig:ks}
\end{figure}

While this method does not necessarily apply to our occurrence rate probability distributions since they are derived mathematically from first principles \citep{kao2020}, we perform this test empirically in order to provide a more quantitative statement about the nature of the occurrence rate probability distributions. To construct empirical cumulative distribution functions for each occurrence rate probability distribution, we first recreate the distribution by drawing 512 (i.e. the number of sampled occurrence rates in the probability calculation) randomly chosen occurrence rates in each sample using \texttt{np.random.choice}, weighed by the probability of that occurrence rate given by the results of our occurrence rate calculation. As seen in Figure \ref{fig:ks}, the empirical probability distributions do indeed match those of the analytical curves. The number of occurrence rates drawn randomly was chosen as to fill in the probability distribution curve to closely match the analytical curves and does not need to match the number of objects in each sample, as the sampling size of occurrence rates in the analytical result is independent of the number of objects originally input into our calculation. That is, we are getting a resultant distribution whether the input sample included 1 or 30 targets, and the goal is to compare the resultant distributions themselves. Therefore, 512 drawn samples is appropriate in order to map the probability distribution curves, which samples 512 occurrence rates.

Since this method includes variable random drawings, we run the KS test on the three empirically drawn samples for 100 iterations. We take the mean of the resulting p-values to be our nominal p-value and the standard deviation to be the error. The results can be seen in Table \ref{tab:ks_results}. We find that the null-hypothesis is rejected in comparing all three of the distributions. Most prominent is the difference between the low-amplitude variability and high-amplitude variability distributions. This furthermore adds to the evidence that a large sample size may be necessary to observationally constrain the mechanism by which high-amplitude variability arises.

\begin{deluxetable}{l c}[h]
\centering
% \tabletypesize{\footnotesize}
\tablecaption{\normalsize{Results of the KS tests comparing the no-variability, low-amplitude variability, and high-amplitude variability occurrence rate probability distributions.} \label{tab:ks_results}}
\tablehead{
% \vspace{-0.3cm}
\colhead{Comparison Samples} & \colhead{p-value}\\
\vspace{-0.4cm}
}
\startdata
No - Low & 0.44E-03 $\pm$ 2.22E-03\\
Low - High & 4.00E-61 $\pm$ 3.95E-60\\
No - High & 5.72E-40 $\pm$ 4.61E-39\\
\enddata
\end{deluxetable}
